# Supplementary material for: MLPST: MLP is All You Need for Spatio-Temporal Prediction
Source: arXiv:2309.13363 source file (2023-09-23)
Supplement: Supplementary file 1 [file 7Appendix.tex]

\newpage

\section{Technical Appendix}
\subsection{Hyper-parameter Tuning}
\label{sub:baselines}
\begin{table}[h]
\centering
\caption{Hyper-parameter search range}
\setlength{\tabcolsep}{0.6mm}{
\begin{tabular}{|c|c|c|}
\hline
Model types & Hyper parameters & Search range \\ \hline
G,L,O,R & learning\_rate (lr) & {[}0.0003,0.0002,0.001,0.01{]} \\
G,O,R & lr\_scheduler & {[}MultiStepLR,StepLR{]} \\
G,O,R & lr\_decary\_ratio & {[}0.1,0.3,0.5,0.7{]} \\
L,O,R & max\_grad\_norm & {[}0.1,5{]} \\
G,R & hidden\_size & {[}16,64,128{]} \\
G,R & num\_layer & {[}1,2{]} \\
L,R & dropout & {[}0,0.2,0.5{]} \\
G & weight\_decay & {[}0.0001,0.001{]} \\ \hline
\end{tabular}}
\label{Table:2}
\end{table}

% \begin{figure*}[t]
%     \centering
%     \includegraphics[scale=0.58]{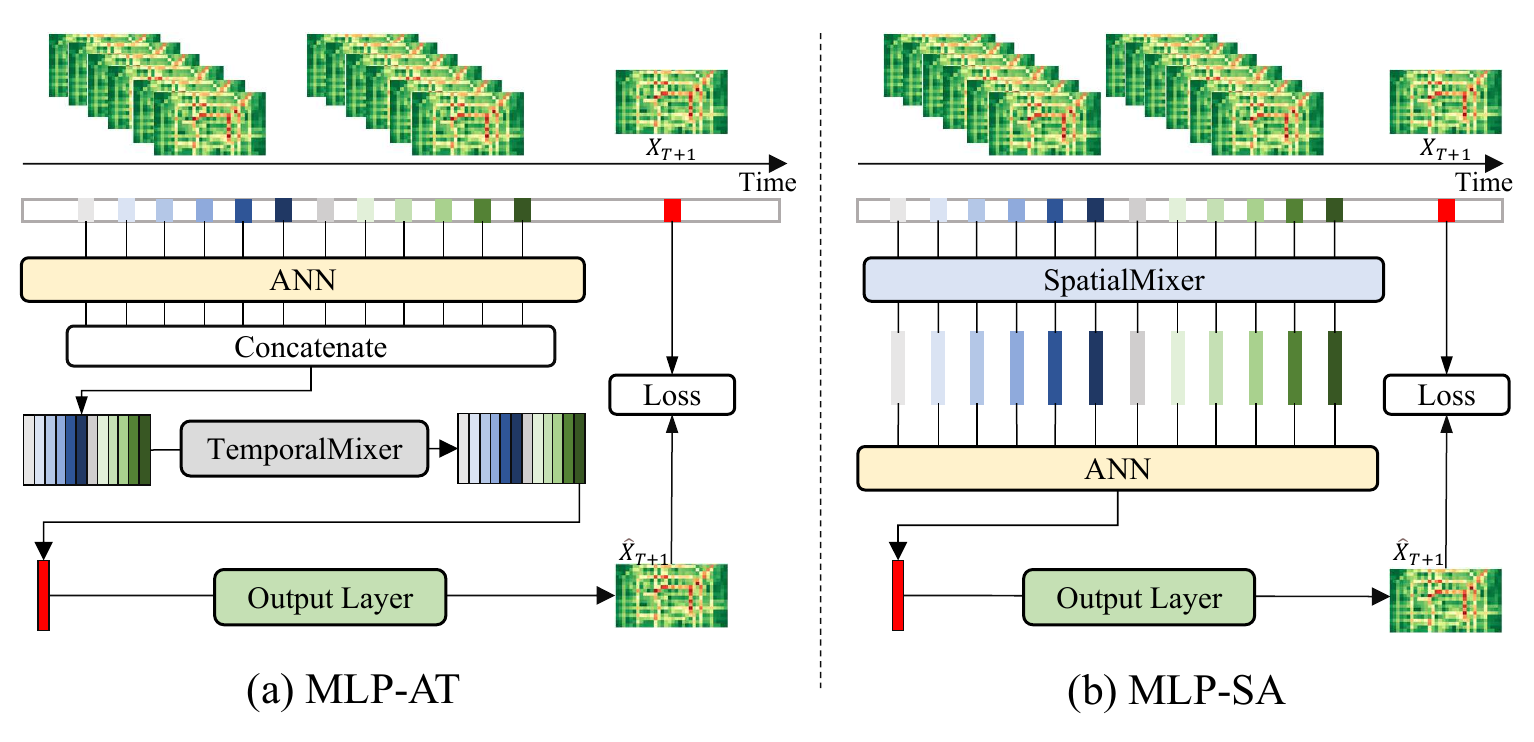}
% % \vspace{-5mm}
%     \caption{Framework demonstration of ablation study.}
%     \label{Fig:Ablation}
% % \vspace{-5mm}
% \end{figure*}

In this subsection, we want to evaluate the performance of all baselines, and tuning the hyperparameters becomes one of the most critical tasks. To show our efforts to tune the baseline models as much as possible while balancing limited computational resources, we list our hyperparameter search ranges and parameter tuning results. As shown in Table \ref{Table:2}, for the sake of simplicity, we divide the baseline and proposed methods into the following subcategories.

\begin{itemize}
\item\textbf{G} includes GCN-based methods, which are ResLSTM, Conv-GCN, Multi-STGCnet.
\item\textbf{L} includes models with long training time, which are ST-ResNet and ACFM.
\item\textbf{O} includes other methods, which is AutoEncoder.
\item\textbf{R} includes RNN-based models, which are FC-RNN and Seq2Seq.
\end{itemize}

As shown in Table \ref{Table:3}, we list out the best hyper-parameters combination from the defined search range under our experimental settings.

% \subsection{Dataset Statistic}
% \label{sub:data}

\begin{table*}[h]
\centering
\caption{Best hyper-parameter results.}
\setlength{\tabcolsep}{0.7mm}{
\begin{tabular}{|c|c|cccccccc|}
\hline
Model & Dataset & lr & lr\_scheduler & lr\_decay\_ratio & max\_grad\_norm & hidden\_size & num\_layer & dropout & weight\_decay \\ \hline
{\color[HTML]{24292F} } & NYCTaxi & 0.01 & multistep & 0.1 & 5 & - & - & 0 & - \\
\multirow{-2}{*}{{\color[HTML]{24292F} AutoEncoder}} & NYCBike & 0.01 & multistep & 0.1 & 5 & - & - & 0 & - \\
 & NYCTaxi & 0.01 & multistep & 0.1 & - & - & - & 0 & - \\
\multirow{-2}{*}{ResLSTM} & NYCBike & 0.01 & multistep & 0.1 & - & - & - & 0 & - \\
{\color[HTML]{404040} } & NYCTaxi & 0.0003 & - & - & - & 16 & - & 0 & - \\
\multirow{-2}{*}{{\color[HTML]{404040} Conv-GCN}} & NYCBike & 0.0003 & - & - & - & 16 & - & 0 & - \\
 & NYCTaxi & 0.001 & StepLR & 0.3 & - & 64 & 1 & 0 & 0.001 \\
\multirow{-2}{*}{Multi-STGCnet} & NYCBike & 0.001 & StepLR & 0.3 & - & 64 & 1 & 0 & 0.001 \\
 & NYCTaxi & 0.0002 & - & - & 0.1 & - & - & 0 & - \\
\multirow{-2}{*}{ST-ResNet} & NYCBike & 0.0002 & - & - & 0.1 & - & - & 0 & - \\
 & NYCTaxi & 0.01 & multisteplr & 0.1 & 5 & 64 & 1 & 0 & - \\
\multirow{-2}{*}{FC-RNN} & NYCBike & 0.01 & multisteplr & 0.1 & 5 & 64 & 1 & 0 & - \\
 & NYCTaxi & 0.01 & multisteplr & 0.1 & 5 & 64 & 1 & 0 & - \\
\multirow{-2}{*}{Seq2Seq} & NYCBike & 0.01 & multisteplr & 0.1 & 5 & 64 & 1 & 0 & - \\
 & NYCTaxi & 0.0003 & - & - & 0.1 & - & - & 0 & - \\
\multirow{-2}{*}{ACFM} & NYCBike & 0.0003 & - & - & 0.1 & - & - & 0.5 & - \\  & NYCTaxi & 0.0003 & - & - & 0.1 & - & - & 0 & - \\
\multirow{-2}{*}{MTGNN} & NYCBike & 0.0003 & - & - & 0.1 & - & - & 0.5 & - \\ \hline
\end{tabular}}
\label{Table:3}
\end{table*}

\subsection{Guidelines for Reproduction}
\label{subsec:guideline}

\subsubsection{Overview}
To facilitate reproduction and fair comparison of a range of model methods across a decade, we store our code in LibCity~\cite{wang2021libcity}. We compare MLPST and other methods on the same dataset with the same split, and keep the same experimental setup at all times. The final results of all experiments are run on one NVIDIA MX330 GPU. Note that the results will not be almost identical for different devices. This is because different devices handle floating-point operations differently\footnote{https://discuss.pytorch.org/t/different-training-results-ondifferent-machines-with-simplified-test-code/59378/3}, even if the pseudo-random generator (seed) is set to be the same.
We compress our code and experimental setup into a zip archive, provided you have a suitable Anaconda environment (preferably the latest version) that supports CUDA (otherwise, there will be no GPU acceleration). The code is a python based on version 3.7, the minimum version of PyTorch is 1.7.1, and the minimum version of cudatoolkit is version 10.2.

Compared to the original LibCity package, our package has the following additions or changes.
\begin{itemize}
\item Full implementation of MLPST and their variants MLP-AT and MLP-SA for ablation studies.
\item Experimental setup files specifying our settings.
\item The processing dataset we use for our experiments.
\end{itemize}
All the above files are accessible, and we do not recommend changing them to prevent unexpected errors. If changes must be made, please follow the documentation available from LibCity\footnote{https://bigscity-libcity-docs.readthedocs.io/zh\_CN/latest/} website.

\subsubsection{Detail usage}
After unpacking, under the "LibCity-MLPST" folder, use pip install -r requirements.txt to install the required packages. After that, you can find the model file you want to copy. For example, if you want to copy MLPST, you can find the "MLPST.py" file and run it using the command python run\_model.py --task traffic\_state\_pred --model MLPST --dataset NYCTaxi20150103, which will automatically call our default hyperparameter model on the NYCTaxi dataset. Suppose you want to try a different hyperparameter or dataset. In that case, you can define an experimental settings file with all the basic settings following LibCity's guidelines or pass it directly from the command line. We provide a default reproduction for each model in both the NYCTaxi and NYCBike datasets. All results shown in Table 1 of the submitted paper are averaged over five runs with the best hyperparameters during the tuning phase. Each run has a unique random seed to avoid bias due to dataset partitioning. If the installation fails or the model does not run successfully, you can follow the LibCity installation guide. After successful installation, add a new model to the model according to LibCity, put the MLPST.py file and MLPST.json in the appropriate locations, then the file you need to modify is libcity/model/traffic\_speed\_prediction/\_\_init\_\_.py to add MLPST to it. Finally, you need to modify some related config files. You need to fix libcity/config/task\_config.json, which is used to set the models and datasets supported by each task and specify the basic parameters the model uses (data module, execution module, evaluation module). Note that if you want to reproduce our results from NYCTaxi and NYCBike, you have to download the processed NYCTaxi and NYCBike dataset atomic files from the LibCity standard dataset and put them in Bigscity-LibCity/raw\_data/dataset\_name, and then you can start experiments. Once the above process is complete, you can start reproducing our results in the NYCTaxi dataset.

\subsubsection{Minimum hardware requirements}
Make sure you have an operating GPU, which is CUDA capable. Also, you need to ensure that your operating system, CUDA driver version, supports PyTorch 1.7.1. 

For reproducing the experiments from NYCBike, we expect most GPUs to function normally. It is expected that most GPUs will run properly. However, if you wish to reproduce the experiments from NYCTaxi, please ensure you have at least 8GB of available GPU memory to operate. Otherwise, we recommend reducing training/evaluation batch size, or reducing embedding size to achieve preferential results.
\subsubsection{Examining the code}
Our code implementations are available for reviewers,
if you wish to examine, their directories are MLPST:
``
LibCity-MLPST$\backslash$libcity$\backslash$model$\backslash$traffic\_flow\_predicion$\backslash$MLPST.py
''
